# Supplementary material for: Observation of spontaneous valley polarization of itinerant electrons
Source: arXiv:2011.06721 ancillary file (2020-11-16)
Supplement: Supplementary file 1 [file SI.2020.Shafayat.valley.AlAs.pdf]

# Supplementary Information: Observation of spontaneous valley polarization of itinerant electrons

Md. S. Hossain, M. K. Ma, K. A. Villegas-Rosales, Y. J. Chung, L. N. Pfeiffer, K. W. West, K. W. Baldwin, and M. Shayegan
*Department of Electrical Engineering, Princeton University, Princeton, New Jersey 08544, USA*
(Dated: November 12, 2020)

## I. EXPERIMENTAL DETAILS

Our material platform is an AlAs quantum well (QW) epitaxially grown via molecular beam epitaxy on a GaAs substrate. The sample contains a 21-nm-wide AlAs QW sandwiched by 68-nm $Al_{0.38}Ga_{0.62}$ barriers. Similar to the case of GaAs, as long as the conduction band offset between the barrier and the QW is sufficiently large, it is possible to confine carriers in the AlAs QW through modulation doping [1–3]. The main difference is that in AlAs the conduction band has lower energy at the X-points of the Brillouin zone instead of the Γ-point. Therefore, the electrons in our AlAs QW are confined in the X-point valleys.

In bulk AlAs, electrons occupy three energetically degenerate ellipsoidal (or six half-ellipsoidal) conduction-band valleys at the six equivalent X-points of the first Brillouin zone [2]. We denote these valleys as X, Y, and Z with the major axes lying along [100], [010], and [001], respectively (see Fig. S1**a**). The electrons in each valley possess an anisotropic Fermi surface with longitudinal and transverse effective masses of $m_l = 1.1$ and $m_t = 0.20$ in units of the free electron mass [2].

When an AlAs QW is formed along the [001] axis, the confinement in the growth direction splits the three-fold valley degeneracy because of the difference in the effective mass along the in-plane and out-of-plane directions. We refer to the out-of-plane valley as Z, and the in-plane valleys as X and Y. At first sight, one would expect that the Z valley should be occupied at all well-widths since it has the larger mass along the confinement direction. However, the slightly larger lattice constant of AlAs compared to GaAs causes biaxial compression in the plane of the AlAs layer, lowering the conduction band of the X and Y valleys relative to the Z valley. This causes the ground-state energies of the two types of valleys to cross at a critical QW width of $\simeq 6$ nm [2]. Above this well-width, the X and Y valleys are occupied; this is the case for our 21-nm-wide AlAs QW (Fig. S1**b**).

In the absence of any additional in-plane strain, electrons in our AlAs QW occupy two in-plane valleys (X and Y) (Fig. S1**b**). This two-fold valley-degeneracy can be lifted via the application of an in-plane, symmetry-breaking, strain $\Delta\varepsilon = \varepsilon_{[100]} - \varepsilon_{[010]}$, where $\varepsilon_{[100]}$ and $\varepsilon_{[010]}$ are the strain values along [100] and [010] [2]. The valley splitting energy is given by $E_V = \varepsilon E_2$, where $E_2$ is the deformation potential, which in AlAs has a band value of 5.8 eV. Positive strain pushes the energy of the X valley up relative to the Y valley, causing electrons to transfer from X to Y, and vice versa for negative strain.

In Fig. S1**c** we show our experimental setup for applying tunable in-plane strain to the two-dimensional electron system (2DES). We glue the sample on one side of a stacked piezoelectric lead-zirconate-titanate actuator with a commercial two-part epoxy [4]. Note in Fig. S1**c** that the sample is glued with its [100] axis along the poling direction of the piezo-actuator. The piezoelectric actuator deforms when a voltage ($V_P$) is applied across its two leads and hence strains the sample glued on top of it. Thus, we introduce nearly uniaxial, in-plane strain to our 2DES. The strain in our sample is $3.6 \times 10^{-7}$ per Volt applied to the piezo-actuator.

It is worthwhile noting that, a finite $V_P$ is required to attain $\varepsilon = 0$ in our experiments [2, 5, 6]. For our sample, this is equal to $-10$ V (see Fig. 2**a**). Such offset in the $\varepsilon = 0$ occurs because of the cooldown- and sample-dependent residual strain originating from the difference in thermal contraction coefficients between the sample, glue, and the piezo-actuator during the cooling process [2, 5, 6].

In order to maintain sufficient strain homogeneity, we used small van der Pauw samples with typical dimensions of 1.5 mm $\times$1.5 mm. Note that the sample edges are along the GaAs cleave directions, [110] and [$\bar{1}$10] (see Fig. S1**d**). The samples are lapped and polished on the back-side down to 150 $\mu$m in order for the strain to propagate to the 2DES efficiently [4]. Electron-beam evaporated Ti-Au alloy on the backside of the sample shields the 2DES from the electric field generated by the applied $V_P$, and also serves as a back gate which we use to change the 2DES density ($n$) *in situ*. Electrical contacts to the 2DES are achieved via alloying a eutectic mixture of In and Sn on the corners and the centers of the sample edges at 425 $^o$C for 270 seconds.

We carried out our experiments in a $^3$He cryostat with a base temperature of $T \simeq 0.30$ K.

## II. MAGNETOTRANSPORT TRACES–INDICATION OF HIGH SAMPLE QUALITY

In the presence of a large perpendicular magnetic field ($B$), the density-of-states for a 2DES splits into a set of discrete Landau levels (LLs). The 2DES hosts different ground states depending on the LL filling factor $\nu$, defined as $\nu = hn/eB$. We show in Fig. S2 magnetoresistance traces as a function of $1/\nu$, taken along the [110] crystallographic direction at $\varepsilon = 0$. Figure S2 traces exhibit well-developed integer quantum Hall states (at $\nu = 1$ and 2) and fractional quantum Hall states (at $\nu = 2/3$ and $1/3$), manifested by pronounced resistance minima, down to very low densities, attesting to the very high quality of our sample. We believe that it is this high quality that allows us to observe the interaction effects in a semicon-

ducting system without being hindered by the single-particle localization by the impurities. This high quality, in turn, leads us to observe and clearly resolve the spontaneous valley polarization.

## III. SPONTANEOUS VALLEY POLARIZATION AND METAL-INSULATOR TRANSITION

In this Section, we examine the temperature dependence of resistance as a function of electron density. Figure S3 shows such data, taken at $\varepsilon = 0$, along the [100] and [010] crystallographic directions. Note that for densities below $n \simeq 6 \times 10^{10}$ cm$^{-2}$ in Fig. S3, $R_{[100]}$ and $R_{[010]}$ are anisotropic and for a given density $R_{[010]} > R_{[100]}$. This is because, as highlighted in the main text, the electrons in our 2DES spontaneously transfer to the Y valley at such densities. Electrons in the Y valley have a small effective mass and therefore higher mobility along [100] [2, 7] which leads to $R_{[010]} > R_{[100]}$.

In the density range $3.2 \times 10^{10}$ cm$^{-2}$ $\lesssim n \lesssim 5.5 \times 10^{10}$ cm$^{-2}$, the resistance decreases with the lowering of temperature, suggesting metallic transport. Below $n \simeq 3.2 \times 10^{10}$ cm$^{-2}$, however, the resistance starts to increase when we lower the temperature, consistent with an insulator. As seen in Figs. S3**a**, **b**, $R_{[100]}$ and $R_{[010]}$ exhibit a similar trend. Therefore, a metal-insulator transition occurs at $n \simeq 3.2 \times 10^{10}$ cm$^{-2}$. Importantly, at the critical density where we observe the spontaneous valley transition, the 2DES still shows metallic behavior. This is in contrast to the critical density for the spontaneous spin transition, $n_S \simeq 2.0 \times 10^{10}$ cm$^{-2}$, where the 2DES is insulating [8].

In Fig. S4, we show a magnified version of Fig. 2**a** data where we plot resistance along [100] and [010] directions as a function of density. Notably, we observe two kinks in $R_{[100]}$ trace (marked with vertical lines) that occur at $n \simeq 3.5$ and 2.0 in units of $10^{10}$ cm$^{-2}$. The locations of these kinks appear to be linked to the critical densities for the metal-insulator and spontaneous spin transitions. It is also clear from Fig. S4 that the spontaneous valley transition occurs at the highest density.

The combination of the experimental results presented in this manuscript and the observations reported in Ref. [8] leads to an experimental phase diagram of the interacting 2DES as a function of the strength of inter-electron interaction, as shown in Fig. S5.

## IV. DATA FROM A SECOND SAMPLE

In this Section, we present data exhibiting the spontaneous valley transition, obtained in a sample taken from a different wafer. This sample contains a slightly narrower (20-nm-thick) QW and a smaller barrier alloy fraction (33%). While we can reach higher densities in this sample, the density cannot be lowered below $n \simeq 3 \times 10^{10}$ cm$^{-2}$ by applying a voltage bias to the backgate.

In Fig. S6 we show resistances along the [100] and [010] directions as function of density, taken at $\varepsilon = 0$. At high densities, the 2DES exhibits isotropic transport, consistent with the valley degeneracy. When we lower the density below $n \simeq 6.9 \times 10^{10}$ cm$^{-2}$, however, $R_{[100]}$ and $R_{[010]}$ separate, signaling a spontaneous splitting of valley degeneracy. This is similar to what we observe for the sample whose data are shown in the main text, but the critical density is $\simeq 10\%$ higher here. This difference might come from the different widths of the AlAs quantum wells in the two samples. Remarkably, similar to Fig. 2, here we also observe that the electrons favor the occupation of the Y valley rather than the X valley once the spontaneous valley transition occurs.

## V. COMPARISON WITH A THEORETICAL PROPOSAL OF SPONTANEOUS VALLEY POLARIZATION IN 2D SYSTEMS WITH ANISOTROPIC EFFECTIVE MASS

A recent theory by Zhu *et al.* [9] predicts that in 2DESs where electrons occupy two valleys with a large effective mass anisotropy, for a sufficiently large anisotropy, the composite fermion Fermi sea at Landau level filling factor $\nu = 1/2$ undergoes a transition to a valley-polarized ground state. The theory does not consider the role of density or $r_s$, and the transition depends only on the mass anisotropy. 2DESs confined to AlAs quantum wells have the required large mass anisotropy, and some of the experimental piezoresistance traces taken as a function of uniaxial, in-plane strain in AlAs 2DESs indeed give a hint of spontaneous valley polarization for composite fermions [9, 10]. However, similar data taken on samples with better quality suggest otherwise [11, 12]. We emphasize that it is not obvious whether there is any connection of this phenomenon to the spontaneous valley transition that we discuss here. In particular, as stated above, the valley polarization considered in Ref. [9] is for composite fermions at high perpendicular magnetic fields, and does not depend on the density or $r_s$ but the valley polarization we report here does.


[1] De Poortere, E. P., Shkolnikov, Y. P., Tutuc, E., Papadakis, S. J. & Shayegan, M. Enhanced electron mobility and high order fractional quantum Hall states in AlAs quantum wells. *Appl. Phys. Lett.* **80**, 1583-1585 (2002).

[2] Shayegan, M., De Poortere, E. P., Gunawan, O., Shkolnikov, Y. P., Tutuc, E. & Vakili, K. Two-dimensional electrons occupying multiple valleys in AlAs. *Phys. Stat. Sol. (b)* **243**, 3629-3642 (2006).

[3] Chung, Y. J., Villegas Rosales, K. A., Deng, H., Baldwin, K. W., West, K. W., Shayegan, M. & Pfeiffer, L. N. Multivalley two-dimensional electron system in an AlAs quantum well with mobility exceeding $2 \times 10^6$ cm$^2$/Vs. *Phys. Rev. Materials* **2**, 071001(R) (2018).

[4] Shayegan, M., Karrai, K., Shkolnikov, Y. P., and Vakili, K., De Poortere, E. P. & Manus, S. Low-temperature, in situ tunable,

uniaxial stress measurements in semiconductors using a piezoelectric actuator. *Appl. Phys. Lett.* **83**, 5235-5237 (2003).

[5] Shkolnikov, Y. P., Vakili, K., De Poortere, E. P. & Shayegan, M. Giant low-temperature piezoresistance effect in AlAs two-dimensional electrons. *Appl. Phys. Lett.* **85**, 3766-3768 (2004).

[6] Gunawan, O., Shkolnikov, Y. P., Vakili, K., Gokmen, T., De Poortere, E. P. & Shayegan, M. Valley susceptibility of an interacting two-dimensional electron system. *Phys. Rev. Lett.* **97**, 186404 (2006).

[7] Gokmen, T., Padmanabhan, Medini & Shayegan, M. Transference of transport anisotropy to composite fermions. *Nat. Phys.* **6**, 621-624 (2010).

[8] Hossain, M. S., Ma, M. K., Villegas Rosales, K. A., Chung, Y. J., Pfeiffer, L. N., West, K. W., Baldwin, K. W. & Shayegan, M. Observation of spontaneous ferromagnetism in a two-dimensional electron system. accepted for publication in *Proc. National Acad. Sci., USA*; cond-mat arXiv:2011.01335.

[9] Z. Zhu, Sheng, D. N., Fu, L. & Sodemann, I. Valley Stoner instability of the composite Fermi sea. *Phys. Rev. B* **98**, 155104 (2018).

[10] Padmanabhan, M., Gokmen, T. & Shayegan, M. Composite fermion valley polarization energies: Evidence for particle-hole asymmetry. *Phys. Rev. B* **81**, 113301 (2010).

[11] Padmanabhan, M. Composite Fermions With A Valley Degree Of Freedom, PhD thesis, Princeton University, 2010; page 55.

[12] Hossain, M. S., Ma, M. K., Pfeiffer, L. N., West, K. W., Baldwin, K. W. & Shayegan, M. unpublished.

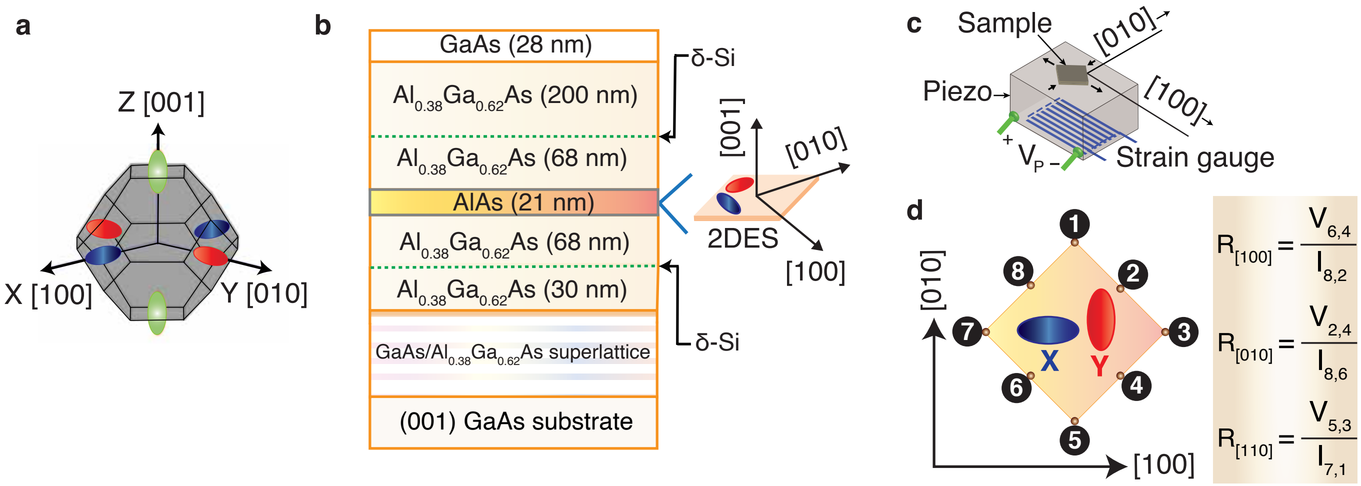


FIG. S1. **a**, First Brillouin zone and constant energy surfaces of the lowest-energy bands for bulk AlAs, showing the X, Y, and Z valleys; [100], [010], and [001] refer to the crystallographic directions. **b**, Structure of our AlAs 2DES grown on a GaAs substrate. The growth direction is [001]. The AlAs layer is under compressive biaxial strain because of the slightly larger lattice constant of AlAs relative to GaAs. This strain results in the occupancy of X and Y valleys only. **c**, Sketch of the experimental setup for applying in-plane strain ($\Delta\varepsilon$). The samples are glued on top of a piezo-actuator, and strain is introduced when a bias voltage ($V_P$) is applied to the actuator's leads. **d**, The sample geometry, including the orientation of the Fermi seas of the two occupied valleys (X and Y), are shown. Contacts to the sample are denoted by 1-8. Measurement configurations for $R_{[100]}$, $R_{[010]}$ and $R_{[110]}$ are also shown.

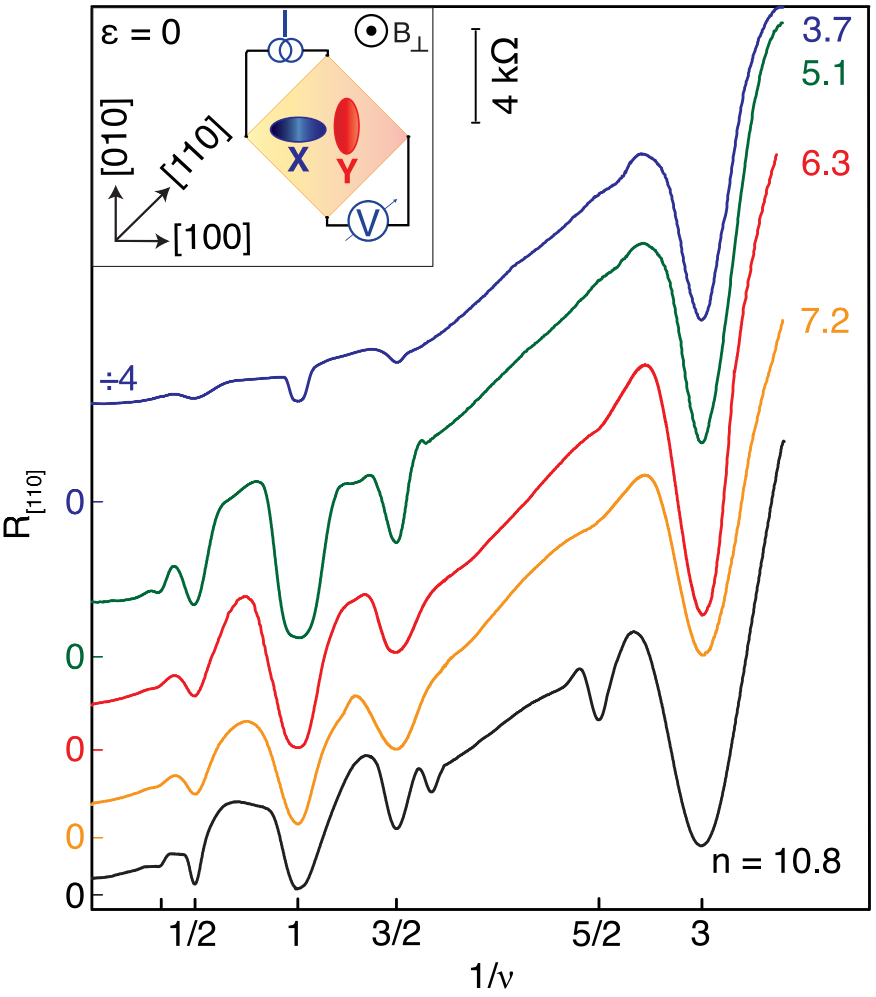


FIG. S2. Magentoresistance traces at $\varepsilon = 0$, taken along [110], plotted against $1/\nu$. The inset captures the sample geometry. Well-developed integer ($\nu = 1, 2$) and fractional ($\nu = 1/3, 2/3$) quantum Hall states are seen over a wide range of densities. The density, in units of $10^{10}$ cm$^{-2}$, is indicated for each trace.

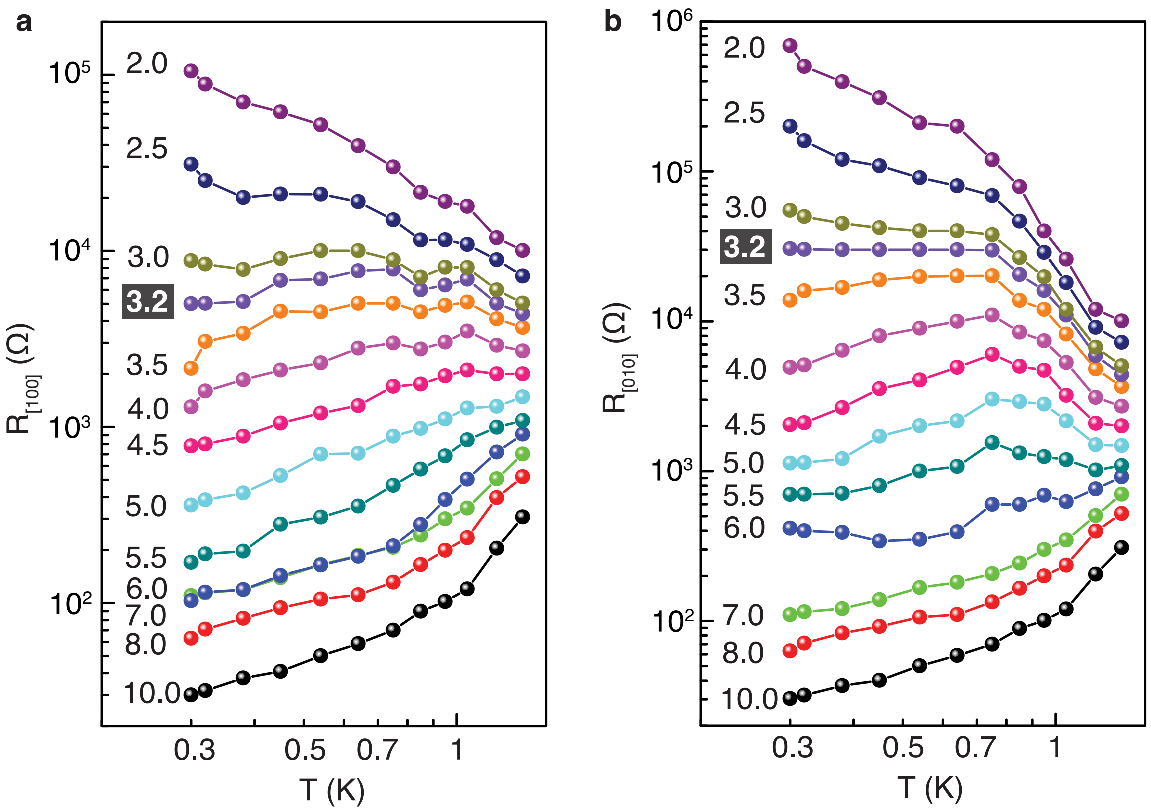


FIG. S3. Longitudinal resistances $R_{[100]}$ and $R_{[010]}$, measured along [100] and [010], respectively, plotted as a function of temperature. Both $R_{[100]}$ and $R_{[010]}$ exhibit metallic transport for $n \geq 3.2 \times 10^{10}$ cm$^{-2}$, and a switch over to an insulating behavior for smaller $n$. This suggests that when the valley transition occurs, the AlAs 2DES is still metallic. The density in units of $10^{10}$ cm$^{-2}$ is given on the left for each trace.

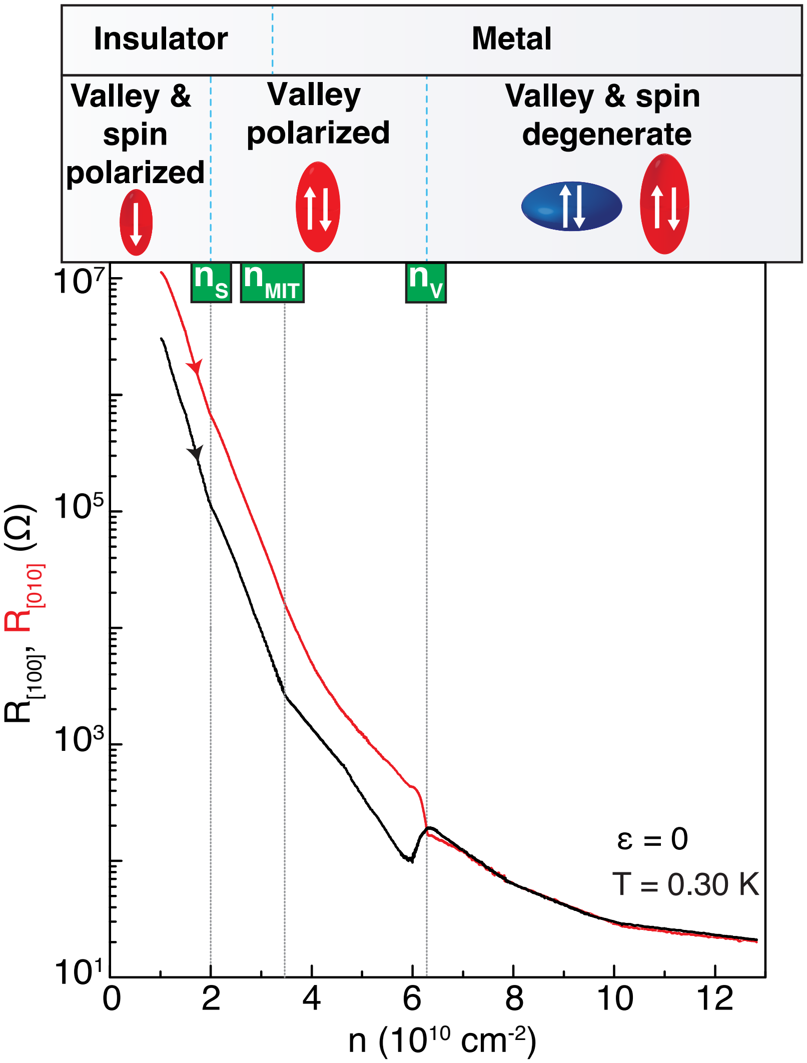


FIG. S4. Same data as in Fig. 2**a** of main text, marking the kinks in $R_{[100]}$ trace. Resistances along [100] and [010] directions at $\varepsilon = 0$ are plotted as a function of density. $R_{[100]}$ and $R_{[010]}$ suddenly split when the spontaneous valley transition occurs at $n_V \simeq 6.3 \times 10^{10}$ cm$^{-2}$. Also, two clear kinks (marked with dotted grey vertical lines) are seen at $n \simeq 3.5$ and 2.0 ($10^{10}$ cm$^{-2}$), which closely correlate with the onset of the metal-insulator transition ($n_{MIT}$) and the spontaneous spin transition $n_S \simeq 2.0 \times 10^{10}$ cm$^{-2}$ [8] (marked with dashed blue vertical lines), respectively.

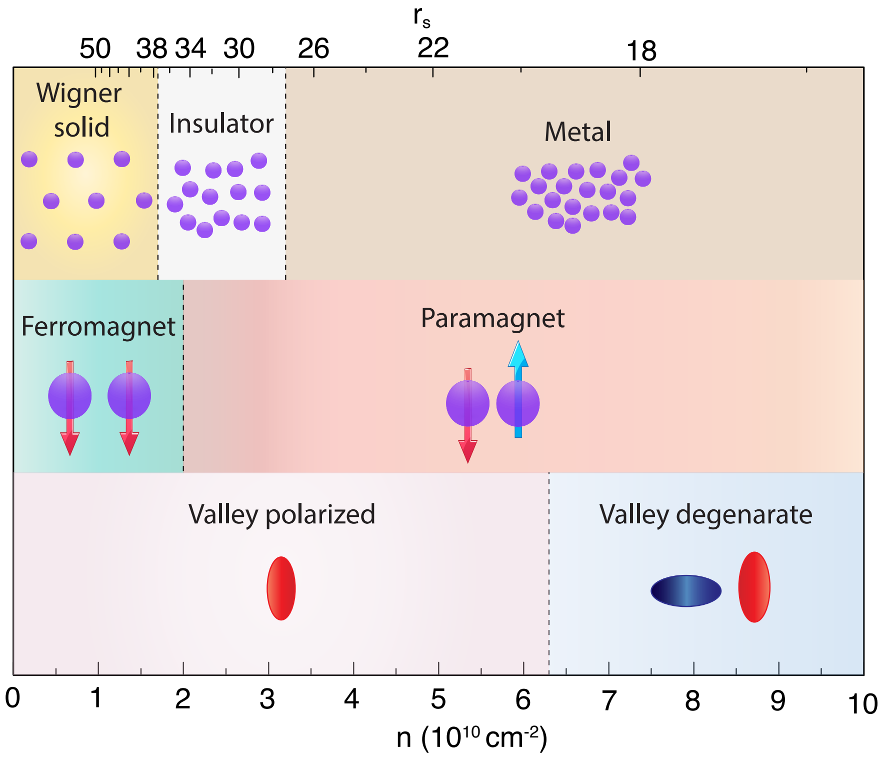


FIG. S5. Full phase diagram for the ground states of an interacting 2DES. The sample is paramagnetic and valley degenerate at high densities. We observe an itinerant transition from a valley-degenerate to a valley-polarized state when the electron density is lowered below a critical value, $n_V = 6.3 \times 10^{10}$ cm$^{-2}$. As detailed in Ref. [8], and shown in Fig. S3, a metal-insulator transition occurs at $n \simeq 3.2 \times 10^{10}$ cm$^{-2}$. As also discussed in Ref. [8], when the density is further lowered, the 2DES makes an abrupt transition to a fully-magnetized state at $n \simeq 2.0 \times 10^{10}$ cm$^{-2}$. At even lower densities, the sample shows signatures of a pinned Wigner solid [8].

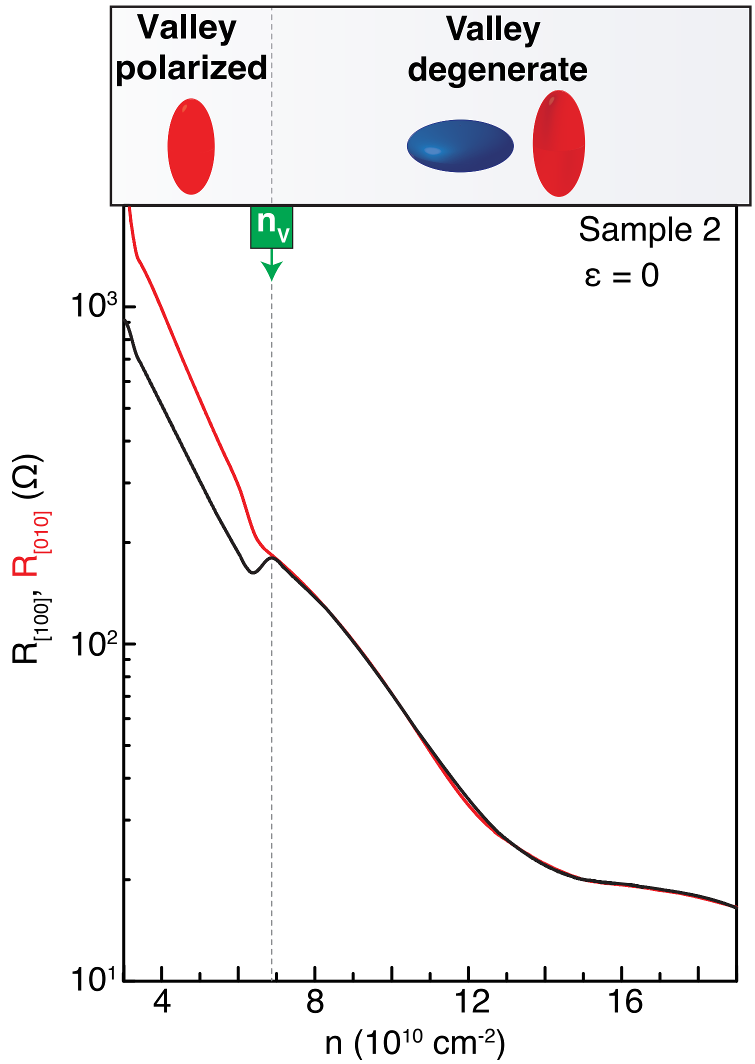


FIG. S6. Signature of spontaneous valley polarization, similar to what is shown in Fig. 2**a** of main text, but here the data are taken from a different AlAs sample, Sample 2. Resistances along [100] and [010] directions at $\varepsilon = 0$ plotted as a function of density. When we lower the density below $n \simeq 7 \times 10^{10}$ cm$^{-2}$, $R_{[100]}$ and $R_{[010]}$ suddenly split, signaling a spontaneous valley transition. The onset density for this transition is slightly ($\simeq 10\%$) larger than that observed in the sample shown in Fig. 2.
